# Supplementary material for: WIT: Wikipedia-based Image Text Dataset for Multimodal Multilingual Machine Learning
Source: arXiv:2103.01913 source file (2021-03-03)
Supplement: Supplementary file 2 [file appendix5.tex]

% Language stats table
% Probably a good idea to include the longtable package.
% Right now, this is split as six tables.

\begin{table*}
  \caption{Language Stats}
  \label{tab:wit-lang-stats-1}
  \begin{tabular}{|c|c|c|c|c|c|c|}
    \hline
    \textbf{Lang}
    & \textbf{Dataset}
    & \textbf{\# Examples}
    & \textbf{\# Uniq. Img}
    & \textbf{\# Ref}
    & \textbf{\# Attr}
    & \textbf{\# Cap}
    \\
  \hline

af & val & 603 & 424 & 371 & 467 & 86 \\
\hline
af & train & 93,755 & 85,728 & 47,173 & 85,180 & 18,403 \\
\hline
af & test & 542 & 497 & 276 & 512 & 116 \\
\hline
an & val & 158 & 127 & 72 & 124 & 43 \\
\hline
an & train & 27,134 & 24,904 & 9,317 & 24,900 & 7,584 \\
\hline
an & test & 186 & 172 & 73 & 178 & 47 \\
\hline
ar & val & 3,888 & 2,630 & 1,520 & 3,173 & 98 \\
\hline
ar & train & 616,618 & 534,440 & 172,069 & 590,016 & 22,228 \\
\hline
ar & test & 3,595 & 3,015 & 1,065 & 3,487 & 134 \\
\hline
arz & val & 1,288 & 1,188 & 68 & 1,262 & 7 \\
\hline
arz & train & 247,771 & 243,215 & 9,387 & 245,931 & 1,700 \\
\hline
arz & test & 1,376 & 1,349 & 64 & 1,364 & 10 \\
\hline
ast & val & 1,091 & 754 & 656 & 800 & 16 \\
\hline
ast & train & 163,466 & 151,164 & 86,392 & 149,505 & 2,385 \\
\hline
ast & test & 978 & 875 & 532 & 930 & 15 \\
\hline
az & val & 752 & 541 & 315 & 608 & 47 \\
\hline
az & train & 122,522 & 109,663 & 34,090 & 117,342 & 9,815 \\
\hline
az & test & 681 & 587 & 206 & 663 & 60 \\
\hline
azb & val & 1,141 & 887 & 308 & 991 & 180 \\
\hline
azb & train & 185,055 & 180,778 & 32,959 & 181,264 & 28,173 \\
\hline
azb & test & 1,080 & 1,035 & 213 & 1,062 & 179 \\
\hline
ba & val & 247 & 187 & 122 & 187 & 43 \\
\hline
ba & train & 39,870 & 37,115 & 16,325 & 37,453 & 7,996 \\
\hline
ba & test & 239 & 214 & 110 & 233 & 35 \\
\hline
bar & val & 199 & 143 & 115 & 141 & 24 \\
\hline
bar & train & 27,762 & 25,995 & 14,813 & 25,307 & 4,551 \\
\hline
bar & test & 177 & 155 & 93 & 168 & 34 \\
\hline
be & val & 896 & 679 & 362 & 763 & 112 \\
\hline
be & train & 147,532 & 129,774 & 51,508 & 138,881 & 19,117 \\
\hline
be & test & 845 & 736 & 308 & 812 & 112 \\
\hline
be-tarask & val & 385 & 285 & 149 & 325 & 38 \\
\hline
be-tarask & train & 64,362 & 56,142 & 22,373 & 60,059 & 7,673 \\
\hline
be-tarask & test & 336 & 303 & 138 & 318 & 46 \\
\hline
bg & val & 2,601 & 1,291 & 1,741 & 1,453 & 153 \\
\hline
bg & train & 282,629 & 246,330 & 137,138 & 257,584 & 29,052 \\
\hline
bg & test & 1,635 & 1,367 & 884 & 1,508 & 169 \\
\hline
bn & val & 643 & 411 & 415 & 467 & 45 \\
\hline
bn & train & 92,497 & 81,882 & 51,035 & 86,040 & 6,670 \\
\hline
bn & test & 590 & 493 & 343 & 563 & 48 \\
\hline
br & val & 435 & 298 & 315 & 299 & 25 \\
\hline
br & train & 65,252 & 60,404 & 41,839 & 55,855 & 4,228 \\
\hline
br & test & 410 & 363 & 279 & 363 & 21 \\
\hline
bs & val & 506 & 339 & 341 & 346 & 48 \\
\hline
bs & train & 72,527 & 66,194 & 39,723 & 65,378 & 8,072 \\
\hline
bs & test & 417 & 374 & 247 & 379 & 52 \\
\hline
ca & val & 4,310 & 2,980 & 1,913 & 3,455 & 267 \\
\hline
ca & train & 698,364 & 592,765 & 246,834 & 654,920 & 53,396 \\
\hline
ca & test & 3,818 & 3,185 & 1,410 & 3,637 & 252 \\
\hline
ce & val & 330 & 308 & 33 & 317 & 272 \\
\hline
ce & train & 54,669 & 54,043 & 2,983 & 54,122 & 47,050 \\
\hline
ce & test & 278 & 276 & 20 & 273 & 237 \\
\hline
ceb & val & 1,467 & 1,278 & 19 & 1,458 & 3 \\
\hline
ceb & train & 273,344 & 251,059 & 3,830 & 272,904 & 2,082 \\
\hline
ceb & test & 1,388 & 1,277 & 17 & 1,386 & 4 \\
\hline
ckb & val & 138 & 76 & 99 & 81 & 11 \\
\hline
ckb & train & 15,424 & 14,321 & 8,811 & 13,800 & 1,283 \\
\hline
ckb & test & 109 & 102 & 65 & 103 & 6 \\
\hline

\end{tabular}
\end{table*}

\begin{table*}
  \caption{Language Stats}
  \label{tab:wit-lang-stats-2}
  \begin{tabular}{|c|c|c|c|c|c|c|}
    \hline
    \textbf{Lang}
    & \textbf{Dataset}
    & \textbf{\# Examples}
    & \textbf{\# Uniq. Img}
    & \textbf{\# Ref}
    & \textbf{\# Attr}
    & \textbf{\# Cap}
    \\
  \hline

cs & val & 4,291 & 2,855 & 2,528 & 3,499 & 877 \\
\hline
cs & train & 652,034 & 557,020 & 332,616 & 613,059 & 147,478 \\
\hline
cs & test & 3,447 & 2,886 & 1,767 & 3,273 & 724 \\
\hline
cv & val & 118 & 89 & 60 & 87 & 18 \\
\hline
cv & train & 14,742 & 14,013 & 6,467 & 13,337 & 1,867 \\
\hline
cv & test & 103 & 96 & 51 & 94 & 11 \\
\hline
cy & val & 773 & 535 & 221 & 656 & 19 \\
\hline
cy & train & 122,238 & 106,448 & 21,917 & 117,650 & 2,966 \\
\hline
cy & test & 720 & 618 & 159 & 697 & 25 \\
\hline
da & val & 1,707 & 1,117 & 1,177 & 1,211 & 79 \\
\hline
da & train & 235,285 & 209,386 & 142,343 & 212,290 & 16,701 \\
\hline
da & test & 1,397 & 1,211 & 864 & 1,272 & 96 \\
\hline
de & val & 23,589 & 13,374 & 14,377 & 17,954 & 3,973 \\
\hline
de & train & 3,350,887 & 2,632,431 & 1,720,948 & 3,192,611 & 721,886 \\
\hline
de & test & 17,507 & 13,205 & 9,413 & 16,806 & 3,539 \\
\hline
el & val & 1,312 & 808 & 766 & 945 & 88 \\
\hline
el & train & 187,283 & 165,482 & 94,120 & 170,918 & 5,664 \\
\hline
el & test & 1,119 & 959 & 589 & 1,055 & 41 \\
\hline
en & val & 45,542 & 19,979 & 33,173 & 29,385 & 3,193 \\
\hline
en & train & 5,422,027 & 3,940,784 & 3,264,650 & 5,094,378 & 561,756 \\
\hline
en & test & 33,177 & 21,870 & 22,439 & 31,699 & 3,662 \\
\hline
eo & val & 1,771 & 1,247 & 1,103 & 1,343 & 232 \\
\hline
eo & train & 286,521 & 254,160 & 156,601 & 260,429 & 44,127 \\
\hline
eo & test & 1,589 & 1,339 & 885 & 1,484 & 265 \\
\hline
es & val & 13,390 & 7,378 & 9,644 & 8,552 & 221 \\
\hline
es & train & 1,741,015 & 1,433,075 & 1,092,875 & 1,530,281 & 37,151 \\
\hline
es & test & 9,876 & 7,658 & 6,461 & 9,001 & 198 \\
\hline
et & val & 1,372 & 771 & 1,009 & 865 & 49 \\
\hline
et & train & 169,304 & 150,267 & 109,891 & 150,847 & 9,761 \\
\hline
et & test & 966 & 835 & 666 & 872 & 50 \\
\hline
eu & val & 1,951 & 1,520 & 549 & 1,715 & 27 \\
\hline
eu & train & 321,311 & 294,256 & 63,662 & 310,440 & 4,914 \\
\hline
eu & test & 1,771 & 1,604 & 393 & 1,731 & 15 \\
\hline
fa & val & 3,162 & 2,215 & 1,305 & 2,562 & 389 \\
\hline
fa & train & 487,183 & 429,833 & 148,916 & 468,121 & 73,117 \\
\hline
fa & test & 2,839 & 2,447 & 962 & 2,758 & 437 \\
\hline
fi & val & 2,493 & 1,709 & 1,490 & 1,846 & 343 \\
\hline
fi & train & 377,569 & 333,999 & 188,244 & 348,713 & 64,404 \\
\hline
fi & test & 2,166 & 1,897 & 1,100 & 2,032 & 401 \\
\hline
fil & val & 273 & 193 & 149 & 221 & 21 \\
\hline
fil & train & 37,964 & 35,009 & 18,968 & 34,446 & 5,221 \\
\hline
fil & test & 353 & 242 & 207 & 269 & 33 \\
\hline
fr & val & 16,822 & 10,221 & 8,243 & 13,463 & 3,579 \\
\hline
fr & train & 2,561,756 & 2,018,324 & 976,576 & 2,444,258 & 658,134 \\
\hline
fr & test & 13,943 & 10,479 & 5,851 & 13,444 & 3,521 \\
\hline
fy & val & 353 & 218 & 248 & 258 & 17 \\
\hline
fy & train & 49,108 & 44,420 & 31,821 & 44,169 & 2,944 \\
\hline
fy & test & 328 & 292 & 227 & 308 & 23 \\
\hline
ga & val & 501 & 159 & 461 & 171 & 6 \\
\hline
ga & train & 33,094 & 31,344 & 25,471 & 28,807 & 1,404 \\
\hline
ga & test & 232 & 217 & 180 & 212 & 9 \\
\hline
gl & val & 1,244 & 743 & 817 & 827 & 36 \\
\hline
gl & train & 176,492 & 151,579 & 96,982 & 157,170 & 6,876 \\
\hline
gl & test & 1,032 & 873 & 579 & 953 & 46 \\
\hline
hi & val & 486 & 327 & 306 & 358 & 24 \\
\hline
hi & train & 69,397 & 61,813 & 38,280 & 62,967 & 4,929 \\
\hline
hi & test & 542 & 448 & 347 & 522 & 54 \\
\hline

\end{tabular}
\end{table*}

\begin{table*}
  \caption{Language Stats}
  \label{tab:wit-lang-stats-3}
  \begin{tabular}{|c|c|c|c|c|c|c|}
    \hline
    \textbf{Lang}
    & \textbf{Dataset}
    & \textbf{\# Examples}
    & \textbf{\# Uniq. Img}
    & \textbf{\# Ref}
    & \textbf{\# Attr}
    & \textbf{\# Cap}
    \\
  \hline

hr & val & 918 & 602 & 615 & 631 & 97 \\
\hline
hr & train & 139,111 & 118,919 & 79,178 & 123,083 & 18,866 \\
\hline
hr & test & 900 & 722 & 541 & 803 & 124 \\
\hline
hsb & val & 91 & 72 & 29 & 85 & 30 \\
\hline
hsb & train & 16,945 & 15,571 & 4,610 & 16,360 & 4,898 \\
\hline
hsb & test & 102 & 92 & 33 & 101 & 32 \\
\hline
ht & val & 142 & 120 & 35 & 119 & 69 \\
\hline
ht & train & 23,751 & 23,376 & 3,745 & 23,305 & 12,889 \\
\hline
ht & test & 148 & 144 & 21 & 147 & 90 \\
\hline
hu & val & 3,655 & 2,564 & 1,654 & 2,969 & 508 \\
\hline
hu & train & 563,738 & 495,429 & 209,013 & 519,752 & 86,780 \\
\hline
hu & test & 3,144 & 2,700 & 1,186 & 2,920 & 465 \\
\hline
hy & val & 1,713 & 1,235 & 670 & 1,379 & 37 \\
\hline
hy & train & 258,993 & 237,008 & 71,621 & 247,576 & 6,886 \\
\hline
hy & test & 1,454 & 1,289 & 419 & 1,401 & 52 \\
\hline
ia & val & 116 & 99 & 17 & 104 & 7 \\
\hline
ia & train & 16,666 & 16,250 & 2,075 & 16,112 & 698 \\
\hline
ia & test & 105 & 100 & 13 & 103 & 8 \\
\hline
id & val & 1,865 & 1,144 & 1,179 & 1,316 & 122 \\
\hline
id & train & 271,133 & 234,762 & 146,112 & 247,845 & 22,030 \\
\hline
id & test & 1,593 & 1,338 & 938 & 1,483 & 143 \\
\hline
io & val & 127 & 84 & 77 & 90 & 20 \\
\hline
io & train & 21,704 & 20,045 & 9,684 & 19,776 & 4,813 \\
\hline
io & test & 143 & 125 & 70 & 133 & 25 \\
\hline
is & val & 242 & 171 & 190 & 165 & 18 \\
\hline
is & train & 35,104 & 32,701 & 24,350 & 30,276 & 3,213 \\
\hline
is & test & 219 & 201 & 167 & 198 & 16 \\
\hline
it & val & 10,111 & 5,858 & 5,990 & 7,236 & 1,126 \\
\hline
it & train & 1,405,878 & 1,155,676 & 649,558 & 1,323,265 & 205,415 \\
\hline
it & test & 7,717 & 6,106 & 3,683 & 7,358 & 1,081 \\
\hline
iw & val & 2,775 & 1,610 & 1,636 & 2,168 & 152 \\
\hline
iw & train & 362,493 & 312,224 & 174,576 & 337,418 & 25,760 \\
\hline
iw & test & 2,091 & 1,740 & 1,052 & 1,949 & 137 \\
\hline
ja & val & 8,851 & 4,313 & 6,410 & 5,367 & 504 \\
\hline
ja & train & 1,084,871 & 874,699 & 624,537 & 1,003,353 & 92,839 \\
\hline
ja & test & 6,023 & 4,647 & 3,598 & 5,590 & 556 \\
\hline
jv & val & 130 & 99 & 83 & 97 & 6 \\
\hline
jv & train & 20,119 & 19,143 & 12,097 & 18,088 & 1,274 \\
\hline
jv & test & 122 & 116 & 73 & 119 & 8 \\
\hline
ka & val & 629 & 468 & 270 & 513 & 29 \\
\hline
ka & train & 104,856 & 94,129 & 36,443 & 97,517 & 8,248 \\
\hline
ka & test & 656 & 566 & 244 & 620 & 63 \\
\hline
kk & val & 325 & 245 & 150 & 266 & 69 \\
\hline
kk & train & 57,517 & 52,867 & 23,358 & 53,446 & 12,249 \\
\hline
kk & test & 336 & 297 & 158 & 320 & 63 \\
\hline
kn & val & 214 & 150 & 160 & 162 & 17 \\
\hline
kn & train & 30,406 & 28,060 & 21,687 & 27,315 & 1,566 \\
\hline
kn & test & 231 & 201 & 184 & 215 & 16 \\
\hline
ko & val & 2,065 & 1,386 & 1,138 & 1,573 & 183 \\
\hline
ko & train & 308,740 & 274,285 & 137,209 & 285,007 & 27,979 \\
\hline
ko & test & 1,802 & 1,586 & 881 & 1,674 & 165 \\
\hline
la & val & 1,209 & 680 & 1,027 & 658 & 96 \\
\hline
la & train & 142,674 & 134,587 & 108,875 & 124,441 & 18,944 \\
\hline
la & test & 742 & 690 & 569 & 674 & 101 \\
\hline
lah & val & 170 & 125 & 70 & 140 & 9 \\
\hline
lah & train & 30,825 & 27,456 & 9,590 & 29,383 & 1,634 \\
\hline
lah & test & 206 & 183 & 69 & 204 & 13 \\
\hline

\end{tabular}
\end{table*}

\begin{table*}
  \caption{Language Stats}
  \label{tab:wit-lang-stats-4}
  \begin{tabular}{|c|c|c|c|c|c|c|}
    \hline
    \textbf{Lang}
    & \textbf{Dataset}
    & \textbf{\# Examples}
    & \textbf{\# Uniq. Img}
    & \textbf{\# Ref}
    & \textbf{\# Attr}
    & \textbf{\# Cap}
    \\
  \hline

lb & val & 324 & 227 & 195 & 243 & 14 \\
\hline
lb & train & 49,401 & 43,998 & 22,042 & 46,565 & 3,278 \\
\hline
lb & test & 274 & 251 & 130 & 260 & 19 \\
\hline
lmo & val & 156 & 122 & 71 & 112 & 31 \\
\hline
lmo & train & 23,815 & 23,058 & 9,675 & 21,607 & 4,387 \\
\hline
lmo & test & 124 & 118 & 56 & 113 & 26 \\
\hline
lt & val & 967 & 723 & 491 & 774 & 77 \\
\hline
lt & train & 150,747 & 137,380 & 62,512 & 139,776 & 12,861 \\
\hline
lt & test & 817 & 728 & 351 & 772 & 71 \\
\hline
lv & val & 609 & 451 & 311 & 501 & 139 \\
\hline
lv & train & 95,165 & 83,567 & 43,276 & 88,648 & 25,237 \\
\hline
lv & test & 573 & 489 & 278 & 522 & 172 \\
\hline
mg & val & 115 & 96 & 41 & 81 & 45 \\
\hline
mg & train & 21,397 & 21,200 & 5,077 & 17,919 & 57 \\
\hline
mg & test & 143 & 142 & 23 & 127 & 15,277 \\
\hline
mk & val & 723 & 485 & 431 & 492 & 75 \\
\hline
mk & train & 113,482 & 97,839 & 59,047 & 103,236 & 25 \\
\hline
mk & test & 676 & 591 & 366 & 626 & 6,041 \\
\hline
ml & val & 564 & 371 & 322 & 424 & 54 \\
\hline
ml & train & 90,149 & 80,683 & 42,723 & 84,472 & 10 \\
\hline
ml & test & 570 & 494 & 292 & 546 & 1,990 \\
\hline
mn & val & 128 & 104 & 73 & 100 & 8 \\
\hline
mn & train & 19,695 & 18,715 & 8,167 & 18,307 & 14 \\
\hline
mn & test & 109 & 102 & 48 & 105 & 1,621 \\
\hline
mr & val & 169 & 131 & 93 & 141 & 6 \\
\hline
mr & train & 24,262 & 22,343 & 12,210 & 22,664 & 63 \\
\hline
mr & test & 165 & 148 & 85 & 162 & 11,330 \\
\hline
ms & val & 728 & 492 & 444 & 562 & 88 \\
\hline
ms & train & 113,190 & 103,204 & 57,894 & 103,981 & 3 \\
\hline
ms & test & 687 & 620 & 389 & 630 & 1,537 \\
\hline
my & val & 107 & 67 & 71 & 79 & 11 \\
\hline
my & train & 17,259 & 16,083 & 10,015 & 15,961 & 739 \\
\hline
my & test & 104 & 97 & 59 & 97 & 131,801 \\
\hline
nan & val & 1,387 & 831 & 603 & 840 & 631 \\
\hline
nan & train & 161,287 & 159,564 & 19,725 & 152,725 & 3 \\
\hline
nan & test & 809 & 792 & 126 & 765 & 888 \\
\hline
nds & val & 144 & 106 & 127 & 99 & 11 \\
\hline
nds & train & 19,024 & 17,954 & 15,735 & 15,998 & 7 \\
\hline
nds & test & 118 & 105 & 97 & 113 & 1,554 \\
\hline
ne & val & 128 & 100 & 66 & 108 & 9 \\
\hline
ne & train & 21,415 & 19,197 & 9,177 & 20,430 & 1,993 \\
\hline
ne & test & 150 & 134 & 72 & 150 & 360,360 \\
\hline
nl & val & 7,888 & 5,014 & 3,434 & 6,524 & 1,825 \\
\hline
nl & train & 1,225,211 & 969,736 & 405,788 & 1,169,330 & 87 \\
\hline
nl & test & 6,511 & 4,975 & 2,300 & 6,244 & 15,892 \\
\hline
nn & val & 796 & 535 & 498 & 589 & 101 \\
\hline
nn & train & 117,036 & 106,463 & 62,556 & 105,519 & 365 \\
\hline
nn & test & 757 & 639 & 413 & 700 & 64,330 \\
\hline
no & val & 2,971 & 1,940 & 1,759 & 2,316 & 452 \\
\hline
no & train & 430,419 & 362,192 & 219,405 & 397,910 & 2 \\
\hline
no & test & 2,662 & 2,072 & 1,510 & 2,496 & 6 \\
\hline
nv & val & 118 & 106 & 20 & 117 & 2,265 \\
\hline
nv & train & 20,691 & 18,386 & 3,300 & 20,479 & 13 \\
\hline
nv & test & 92 & 83 & 21 & 89 & 5 \\
\hline
oc & val & 347 & 251 & 215 & 249 & 1,354 \\
\hline
oc & train & 62,915 & 59,145 & 32,093 & 56,856 & 22 \\
\hline
oc & test & 363 & 326 & 209 & 325 & 2,790 \\
\hline

\end{tabular}
\end{table*}

\begin{table*}
  \caption{Language Stats}
  \label{tab:wit-lang-stats-5}
  \begin{tabular}{|c|c|c|c|c|c|c|}
    \hline
    \textbf{Lang}
    & \textbf{Dataset}
    & \textbf{\# Examples}
    & \textbf{\# Uniq. Img}
    & \textbf{\# Ref}
    & \textbf{\# Attr}
    & \textbf{\# Cap}
    \\
  \hline

pa & val & 193 & 127 & 126 & 136 & 505,890 \\
\hline
pa & train & 27,122 & 25,126 & 15,053 & 25,113 & 2,642 \\
\hline
pa & test & 211 & 184 & 120 & 206 & 416 \\
\hline
pl & val & 7,036 & 4,773 & 3,308 & 5,783 & 73,480 \\
\hline
pl & train & 1,114,489 & 938,346 & 429,129 & 1,054,164 & 396 \\
\hline
pl & test & 5,747 & 4,798 & 2,235 & 5,507 & 16 \\
\hline
pt & val & 6,515 & 3,354 & 3,920 & 4,134 & 3,093 \\
\hline
pt & train & 804,395 & 672,754 & 332,753 & 754,910 & 26 \\
\hline
pt & test & 4,592 & 3,684 & 2,017 & 4,372 & 544 \\
\hline
qu & val & 117 & 75 & 61 & 94 & 102,809 \\
\hline
qu & train & 18,900 & 15,381 & 8,596 & 17,116 & 540 \\
\hline
qu & test & 134 & 103 & 65 & 128 & 797 \\
\hline
ro & val & 2,294 & 1,636 & 924 & 1,939 & 141,748 \\
\hline
ro & train & 375,263 & 324,990 & 116,427 & 357,865 & 764 \\
\hline
ro & test & 2,095 & 1,772 & 719 & 2,013 & 43 \\
\hline
ru & val & 9,808 & 6,225 & 4,445 & 8,067 & 8,537 \\
\hline
ru & train & 1,534,893 & 1,240,599 & 569,666 & 1,467,699 & 54 \\
\hline
ru & test & 8,780 & 6,792 & 3,610 & 8,485 & 7 \\
\hline
sco & val & 329 & 240 & 208 & 246 & 1,073 \\
\hline
sco & train & 47,619 & 45,243 & 28,392 & 42,170 & 12 \\
\hline
sco & test & 304 & 277 & 197 & 275 & 330 \\
\hline
si & val & 95 & 66 & 68 & 63 & 66,022 \\
\hline
si & train & 14,903 & 13,392 & 9,344 & 13,250 & 326 \\
\hline
si & test & 124 & 108 & 76 & 115 & 131 \\
\hline
sk & val & 1,433 & 1,111 & 520 & 1,234 & 27,002 \\
\hline
sk & train & 229,755 & 209,237 & 62,766 & 218,817 & 167 \\
\hline
sk & test & 1,233 & 1,087 & 385 & 1,180 & 59 \\
\hline
sl & val & 1,055 & 673 & 638 & 746 & 11,113 \\
\hline
sl & train & 146,551 & 130,395 & 71,919 & 134,643 & 51 \\
\hline
sl & test & 839 & 735 & 429 & 793 & 100 \\
\hline
sq & val & 355 & 262 & 214 & 263 & 18,810 \\
\hline
sq & train & 48,942 & 44,433 & 22,455 & 45,258 & 103 \\
\hline
sq & test & 273 & 243 & 133 & 252 & 58 \\
\hline
sr & val & 2,649 & 1,538 & 1,617 & 1,719 & 11,953 \\
\hline
sr & train & 358,505 & 314,625 & 166,598 & 324,088 & 81 \\
\hline
sr & test & 2,000 & 1,720 & 1,010 & 1,827 & 450 \\
\hline
sr-Latn & val & 1,007 & 723 & 563 & 707 & 87,196 \\
\hline
sr-Latn & train & 165,373 & 150,072 & 75,782 & 143,264 & 520 \\
\hline
sr-Latn & test & 957 & 840 & 463 & 847 & 11 \\
\hline
sv & val & 6,330 & 4,058 & 3,252 & 4,817 & 2,259 \\
\hline
sv & train & 918,732 & 791,029 & 363,165 & 877,774 & 10 \\
\hline
sv & test & 4,914 & 4,171 & 2,130 & 4,732 & 33 \\
\hline
sw & val & 201 & 136 & 153 & 131 & 5,963 \\
\hline
sw & train & 28,993 & 27,225 & 22,141 & 24,424 & 31 \\
\hline
sw & test & 164 & 151 & 131 & 145 & 17 \\
\hline
ta & val & 608 & 362 & 410 & 424 & 2,501 \\
\hline
ta & train & 85,453 & 75,394 & 48,154 & 77,670 & 17 \\
\hline
ta & test & 526 & 446 & 318 & 496 & 11 \\
\hline
te & val & 279 & 160 & 190 & 189 & 1,823 \\
\hline
te & train & 37,589 & 33,063 & 23,336 & 34,776 & 14 \\
\hline
te & test & 267 & 223 & 168 & 255 & 37 \\
\hline
tg & val & 155 & 125 & 57 & 132 & 8,480 \\
\hline
tg & train & 22,594 & 21,557 & 6,660 & 21,883 & 58 \\
\hline
tg & test & 143 & 137 & 38 & 142 & 142 \\
\hline
th & val & 793 & 544 & 437 & 579 & 25,437 \\
\hline
th & train & 120,592 & 105,618 & 54,853 & 110,325 & 151 \\
\hline
th & test & 750 & 633 & 366 & 697 & 12 \\
\hline

\end{tabular}
\end{table*}

\begin{table*}
  \caption{Language Stats}
  \label{tab:wit-lang-stats-6}
  \begin{tabular}{|c|c|c|c|c|c|c|}
    \hline
    \textbf{Lang}
    & \textbf{Dataset}
    & \textbf{\# Examples}
    & \textbf{\# Uniq. Img}
    & \textbf{\# Ref}
    & \textbf{\# Attr}
    & \textbf{\# Cap}
    \\
  \hline

tr & val & 1,840 & 1,265 & 1,023 & 1,413 & 2,340 \\
\hline
tr & train & 270,292 & 237,703 & 126,042 & 250,380 & 10 \\
\hline
tr & test & 1,591 & 1,366 & 762 & 1,509 & 430 \\
\hline
tt & val & 274 & 225 & 85 & 242 & 78,021 \\
\hline
tt & train & 44,622 & 42,005 & 9,852 & 42,849 & 464 \\
\hline
tt & test & 285 & 268 & 74 & 274 & 173 \\
\hline
uk & val & 5,990 & 4,135 & 2,316 & 4,983 & 27,968 \\
\hline
uk & train & 924,811 & 787,944 & 279,548 & 885,861 & 176 \\
\hline
uk & test & 4,985 & 4,177 & 1,503 & 4,837 & 165 \\
\hline
ur & val & 567 & 413 & 291 & 475 & 27,394 \\
\hline
ur & train & 91,264 & 82,093 & 36,659 & 86,497 & 142 \\
\hline
ur & test & 580 & 489 & 246 & 558 & 251 \\
\hline
uz & val & 272 & 243 & 64 & 249 & 42,060 \\
\hline
uz & train & 42,808 & 42,084 & 7,722 & 41,971 & 205 \\
\hline
uz & test & 239 & 238 & 59 & 239 & 310 \\
\hline
vec & val & 290 & 268 & 25 & 278 & 61,086 \\
\hline
vec & train & 48,684 & 48,262 & 3,728 & 47,735 & 330 \\
\hline
vec & test & 265 & 264 & 40 & 256 & 3 \\
\hline
vi & val & 3,351 & 2,321 & 1,467 & 2,719 & 619 \\
\hline
vi & train & 515,937 & 453,326 & 177,565 & 491,288 & 4 \\
\hline
vi & test & 2,696 & 2,311 & 1,051 & 2,593 & 18 \\
\hline
vo & val & 180 & 157 & 167 & 86 & 4,636 \\
\hline
vo & train & 30,564 & 29,293 & 27,485 & 16,248 & 17 \\
\hline
vo & test & 134 & 127 & 116 & 83 & 2 \\
\hline
war & val & 443 & 354 & 72 & 400 & 1,213 \\
\hline
war & train & 75,167 & 68,979 & 9,022 & 71,917 & 13 \\
\hline
war & test & 334 & 312 & 45 & 316 & 11 \\
\hline
xmf & val & 86 & 77 & 33 & 68 & 1,807 \\
\hline
xmf & train & 15,221 & 14,405 & 5,562 & 13,801 & 11 \\
\hline
xmf & test & 92 & 89 & 27 & 89 & 292 \\
\hline
yue & val & 333 & 260 & 243 & 255 & 58,212 \\
\hline
yue & train & 52,494 & 49,464 & 34,196 & 46,744 & 357 \\
\hline
yue & test & 309 & 293 & 215 & 286 & 291 \\
\hline
zh & val & 5,493 & 3,504 & 3,164 & 4,306 & 58,289 \\
\hline
zh & train & 834,324 & 691,440 & 411,939 & 784,829 & 358 \\
\hline
zh & test & 4,947 & 3,905 & 2,733 & 4,716 &  \\
\hline
zh-TW & val & 5,493 & 3,508 & 3,157 & 4,312 &  \\
\hline
zh-TW & train & 834,941 & 691,337 & 412,317 & 785,378 &  \\
\hline
zh-TW & test & 4,955 & 3,903 & 2,736 & 4,721 &  \\
\hline

\end{tabular}
\end{table*}
